# Supplementary material for: Neural Image Compression with Text-guided Encoding for both Pixel-level and Perceptual Fidelity
Source: arXiv:2403.02944 source file (2024-05-22)
Supplement: Supplementary file 1 [file Appendix_Ours_vs_TGIC.tex]

\begin{figure}[h]
    \setlength{\tabcolsep}{1pt}
    \begin{tabular}{ccc}
    \includegraphics[width=0.32\textwidth ]{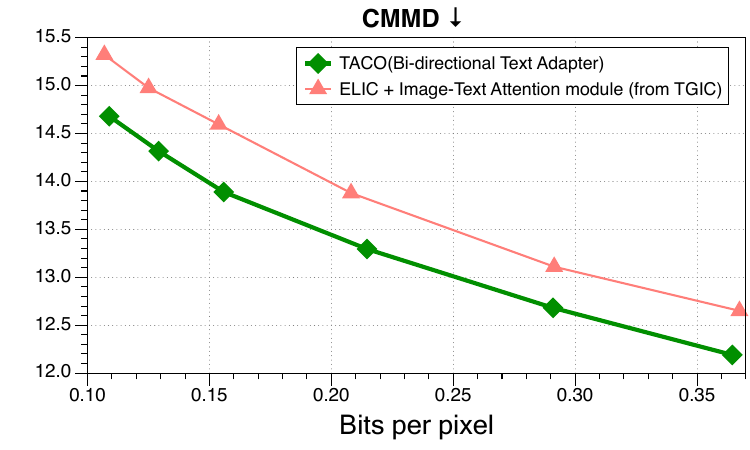}& 
    \includegraphics[width=0.32\textwidth ]{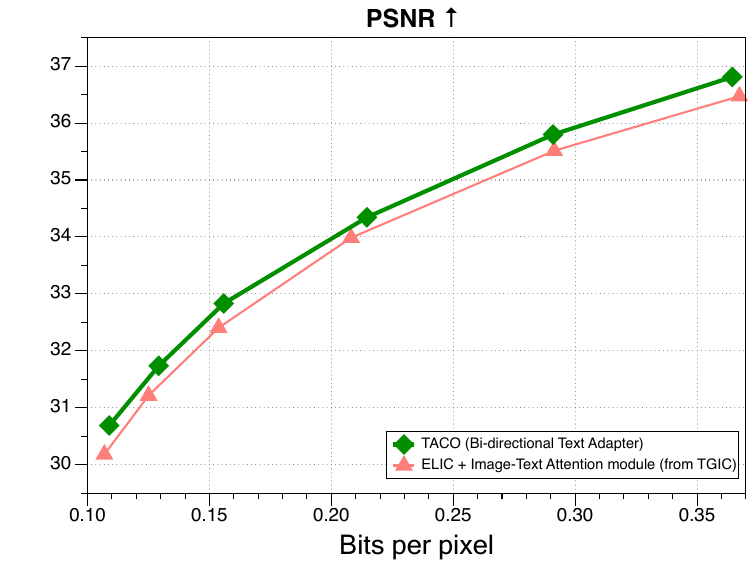}&
    \includegraphics[width=0.32\textwidth ]{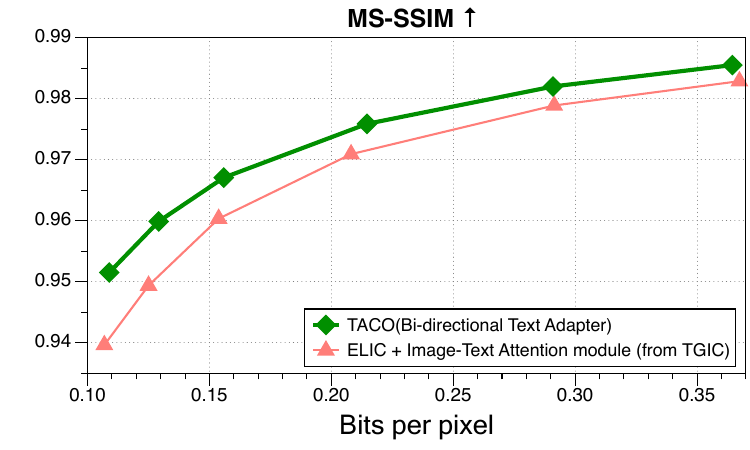}
    \end{tabular}
    \caption{Ablation result:}
    \label{fig:uni_TGIC_appendix}
\end{figure}
