# Supplementary material for: Neural Image Compression with Text-guided Encoding for both Pixel-level and Perceptual Fidelity
Source: arXiv:2403.02944 source file (2024-05-22)
Supplement: Supplementary file 2 [file Appendix_caption_GPT4.tex]

\begin{figure}[h]
    \setlength{\tabcolsep}{1pt}
    \begin{tabular}{ccc}
    \centering
    \includegraphics[width=0.5\textwidth ]{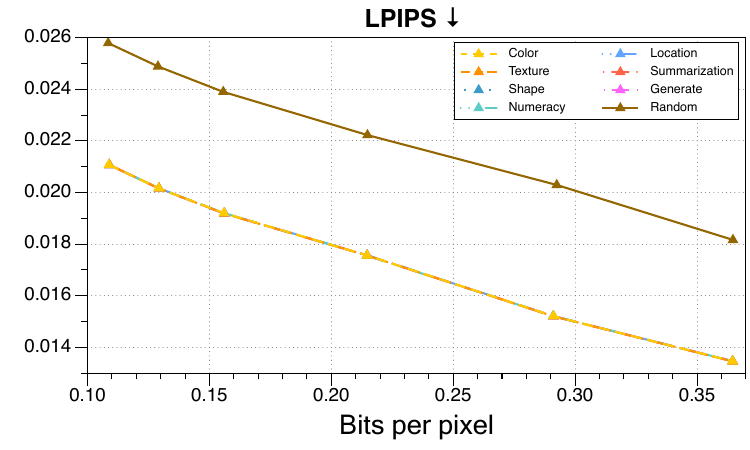}& 
    \includegraphics[width=0.5\textwidth ]{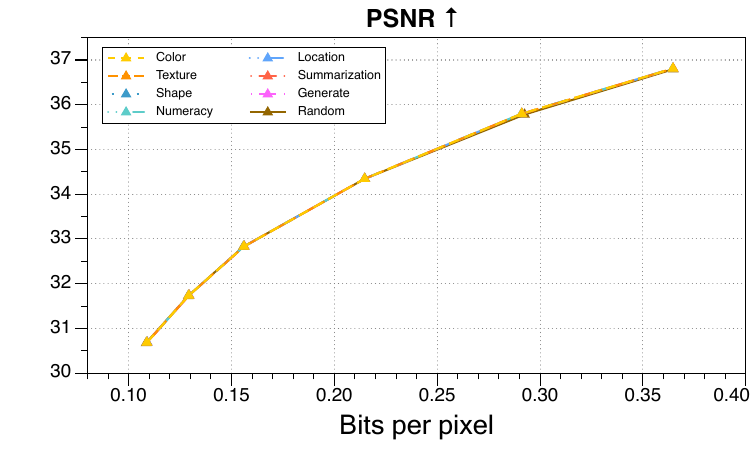}\\
    \includegraphics[width=0.5\textwidth ]{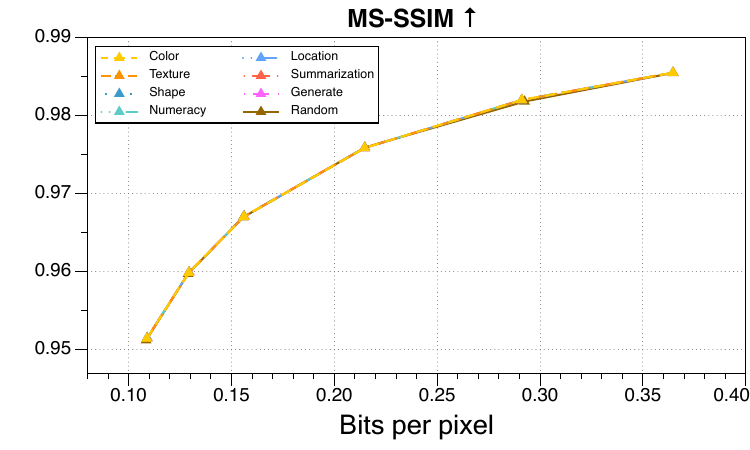}&
    \includegraphics[width=0.5\textwidth ]{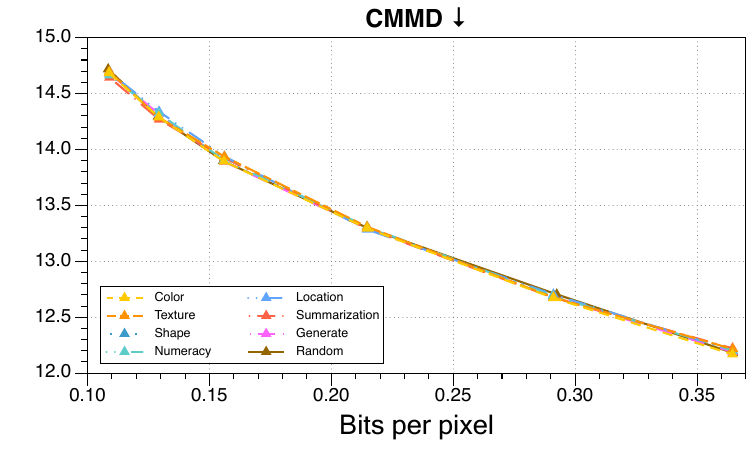}
    \end{tabular}
    \caption{Ablation result: modifying the captions using GPT4}
    \label{fig:gpt4_caption_append}
\end{figure}
