# Supplementary material for: Neural Image Compression with Text-guided Encoding for both Pixel-level and Perceptual Fidelity
Source: arXiv:2403.02944 source file (2024-05-22)
Supplement: Supplementary file 3 [file Appendix_loss_coeff.tex]

\begin{figure}[h]
    \centering
    \begin{tabular}{ccc}
    \includegraphics[width=0.32\textwidth ]{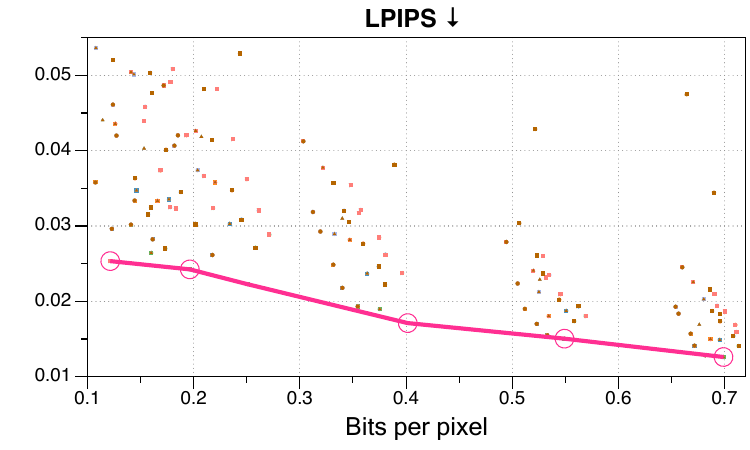}&
    \includegraphics[width=0.32\textwidth ]{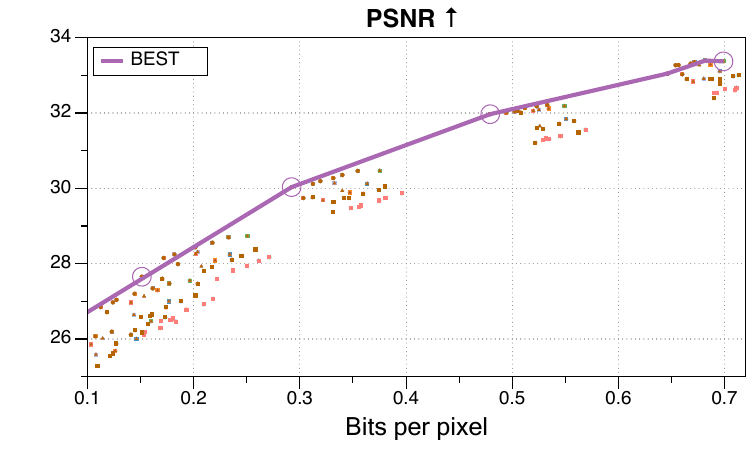}& \includegraphics[width=0.32\textwidth ]{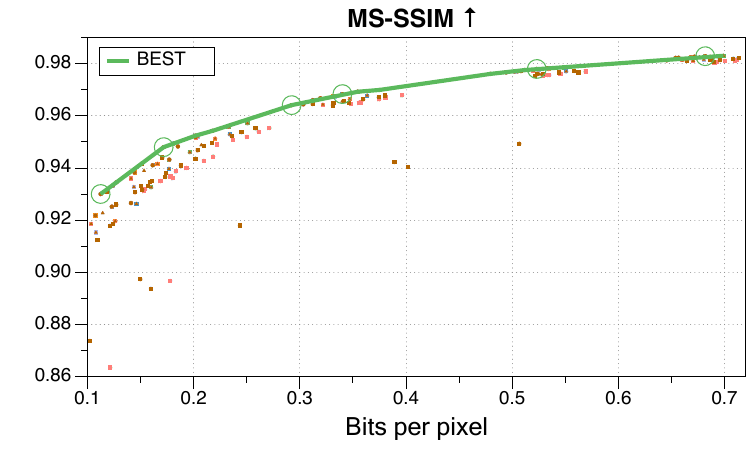}\\
    \end{tabular}
    \caption{Ablation result: }
    \label{fig:loss_coefficient_appen} 
\end{figure}
