# Supplementary material for: Neural Image Compression with Text-guided Encoding for both Pixel-level and Perceptual Fidelity
Source: arXiv:2403.02944 source file (2024-05-22)
Supplement: Supplementary file 5 [file Appendix_qualitative_clic_net.tex]

\begin{figure*}[!h]
    \centering
    {\includegraphics[width=0.87\columnwidth]{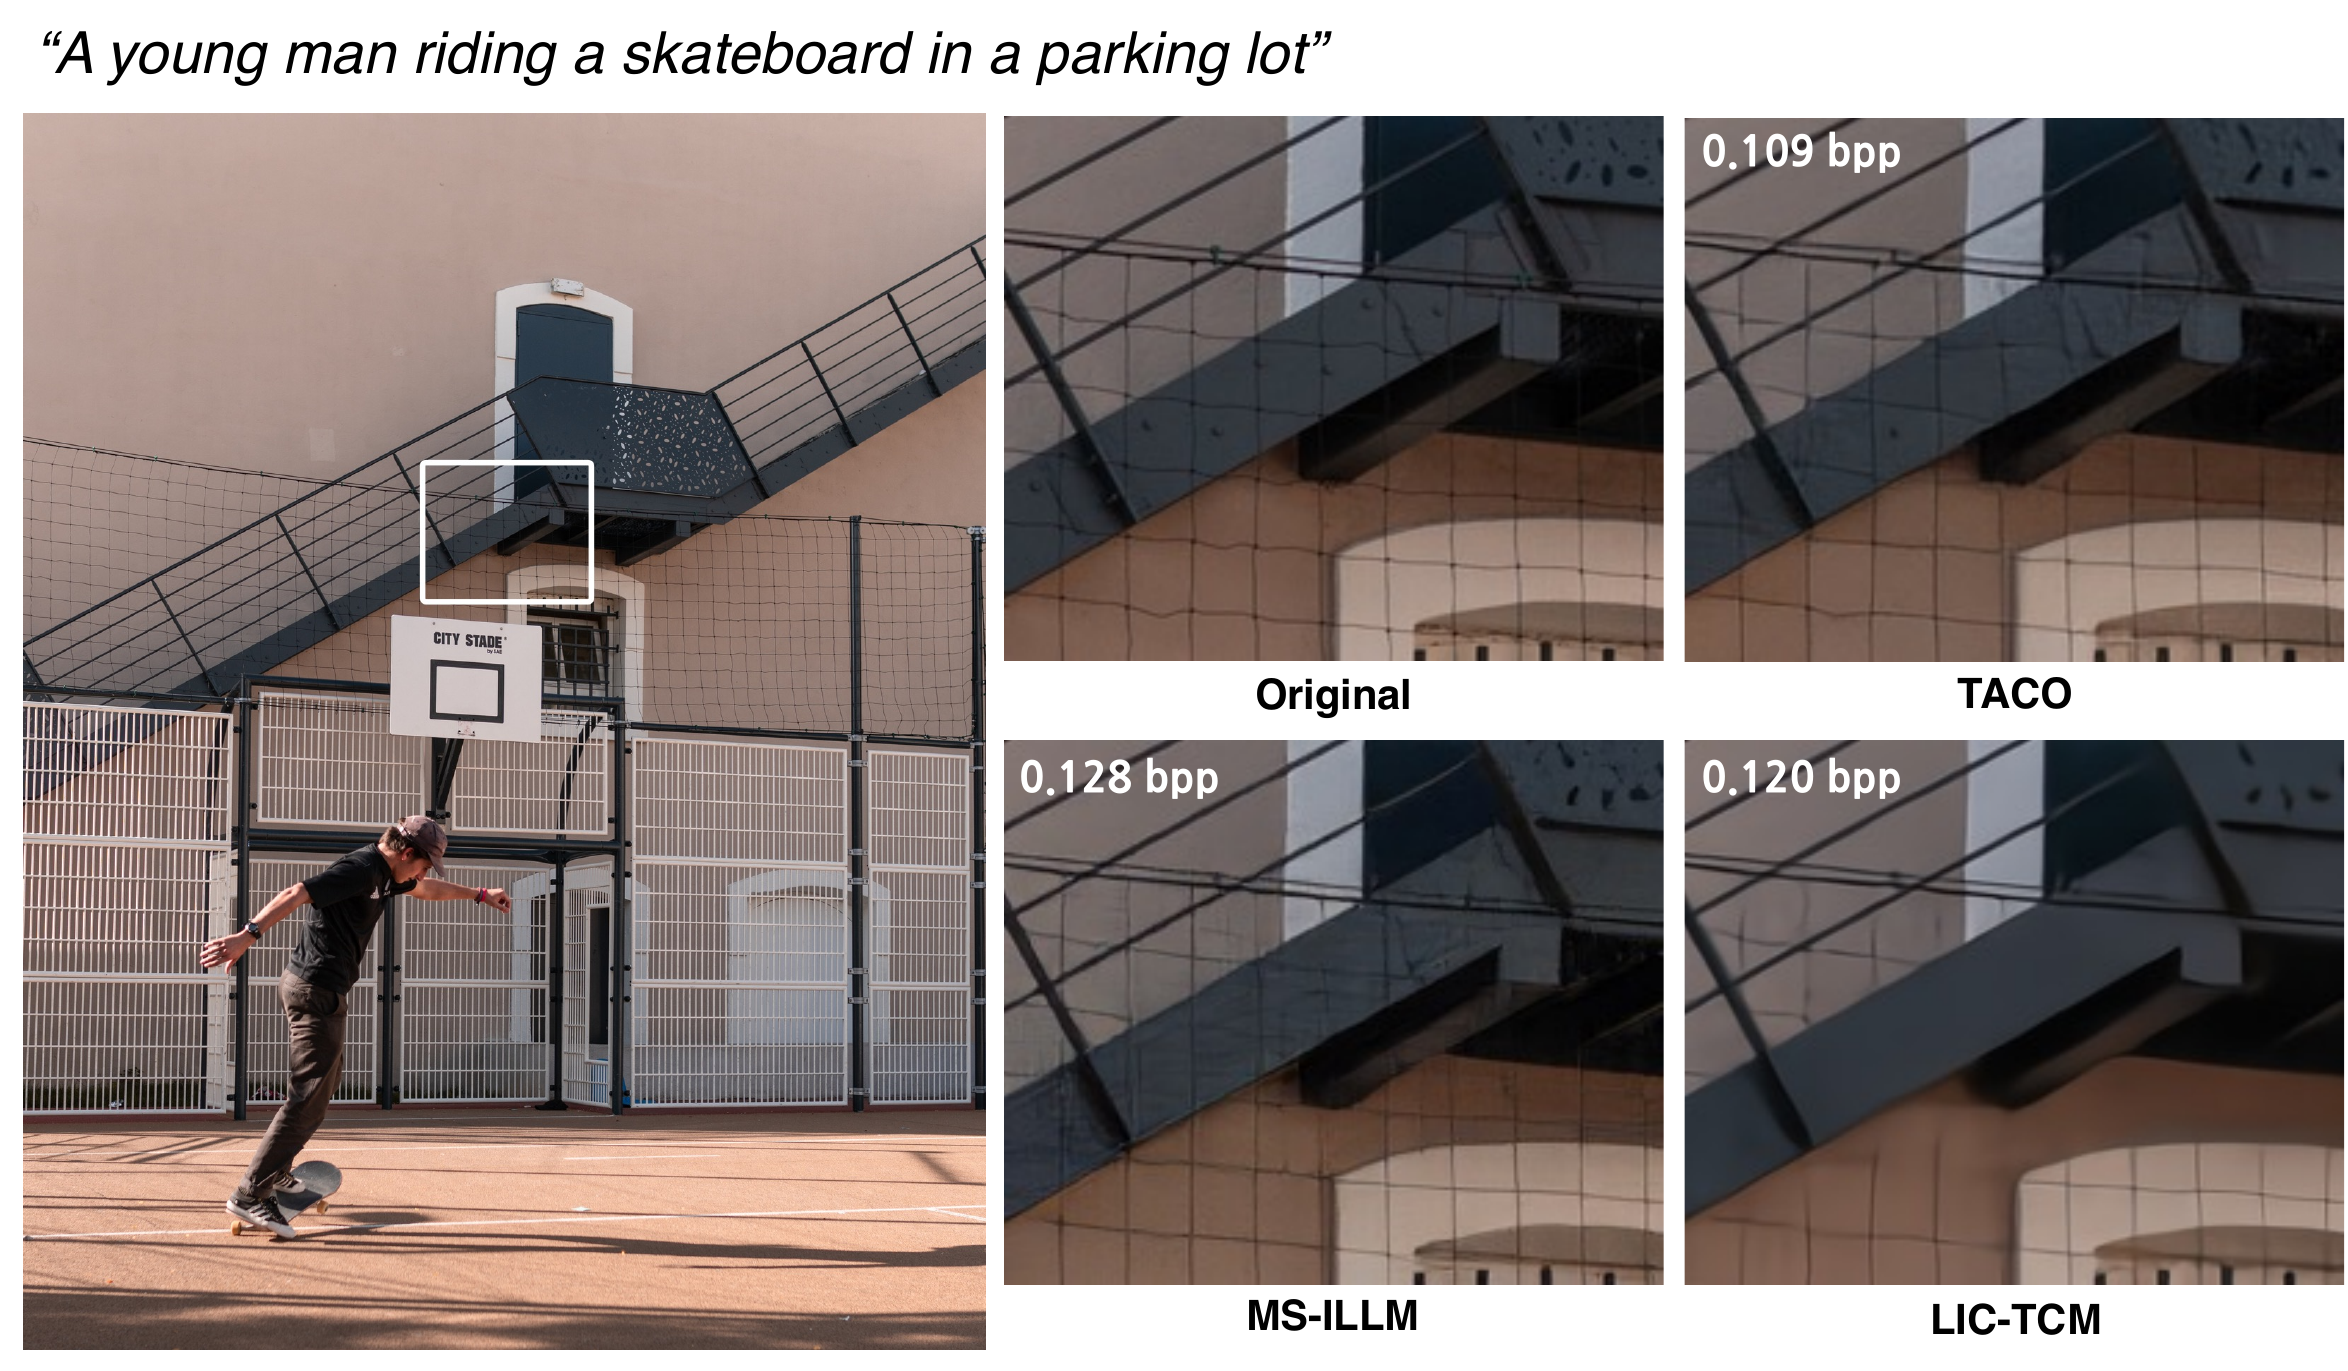}}
    \caption{ \textbf{Qualitative results.} TACO generate more information-preserved image conditioned on given captions. The quality of reconstructed net is a good evidence for this. }
    \label{fig:appendix_qualitative_net} 
\end{figure*}
