# Supplementary material for: Neural Image Compression with Text-guided Encoding for both Pixel-level and Perceptual Fidelity
Source: arXiv:2403.02944 source file (2024-05-22)
Supplement: Supplementary file 6 [file Appendix_qualitative_clic_piano.tex]

\begin{figure*}[!h]
    \centering
    {\includegraphics[width=0.87\columnwidth]{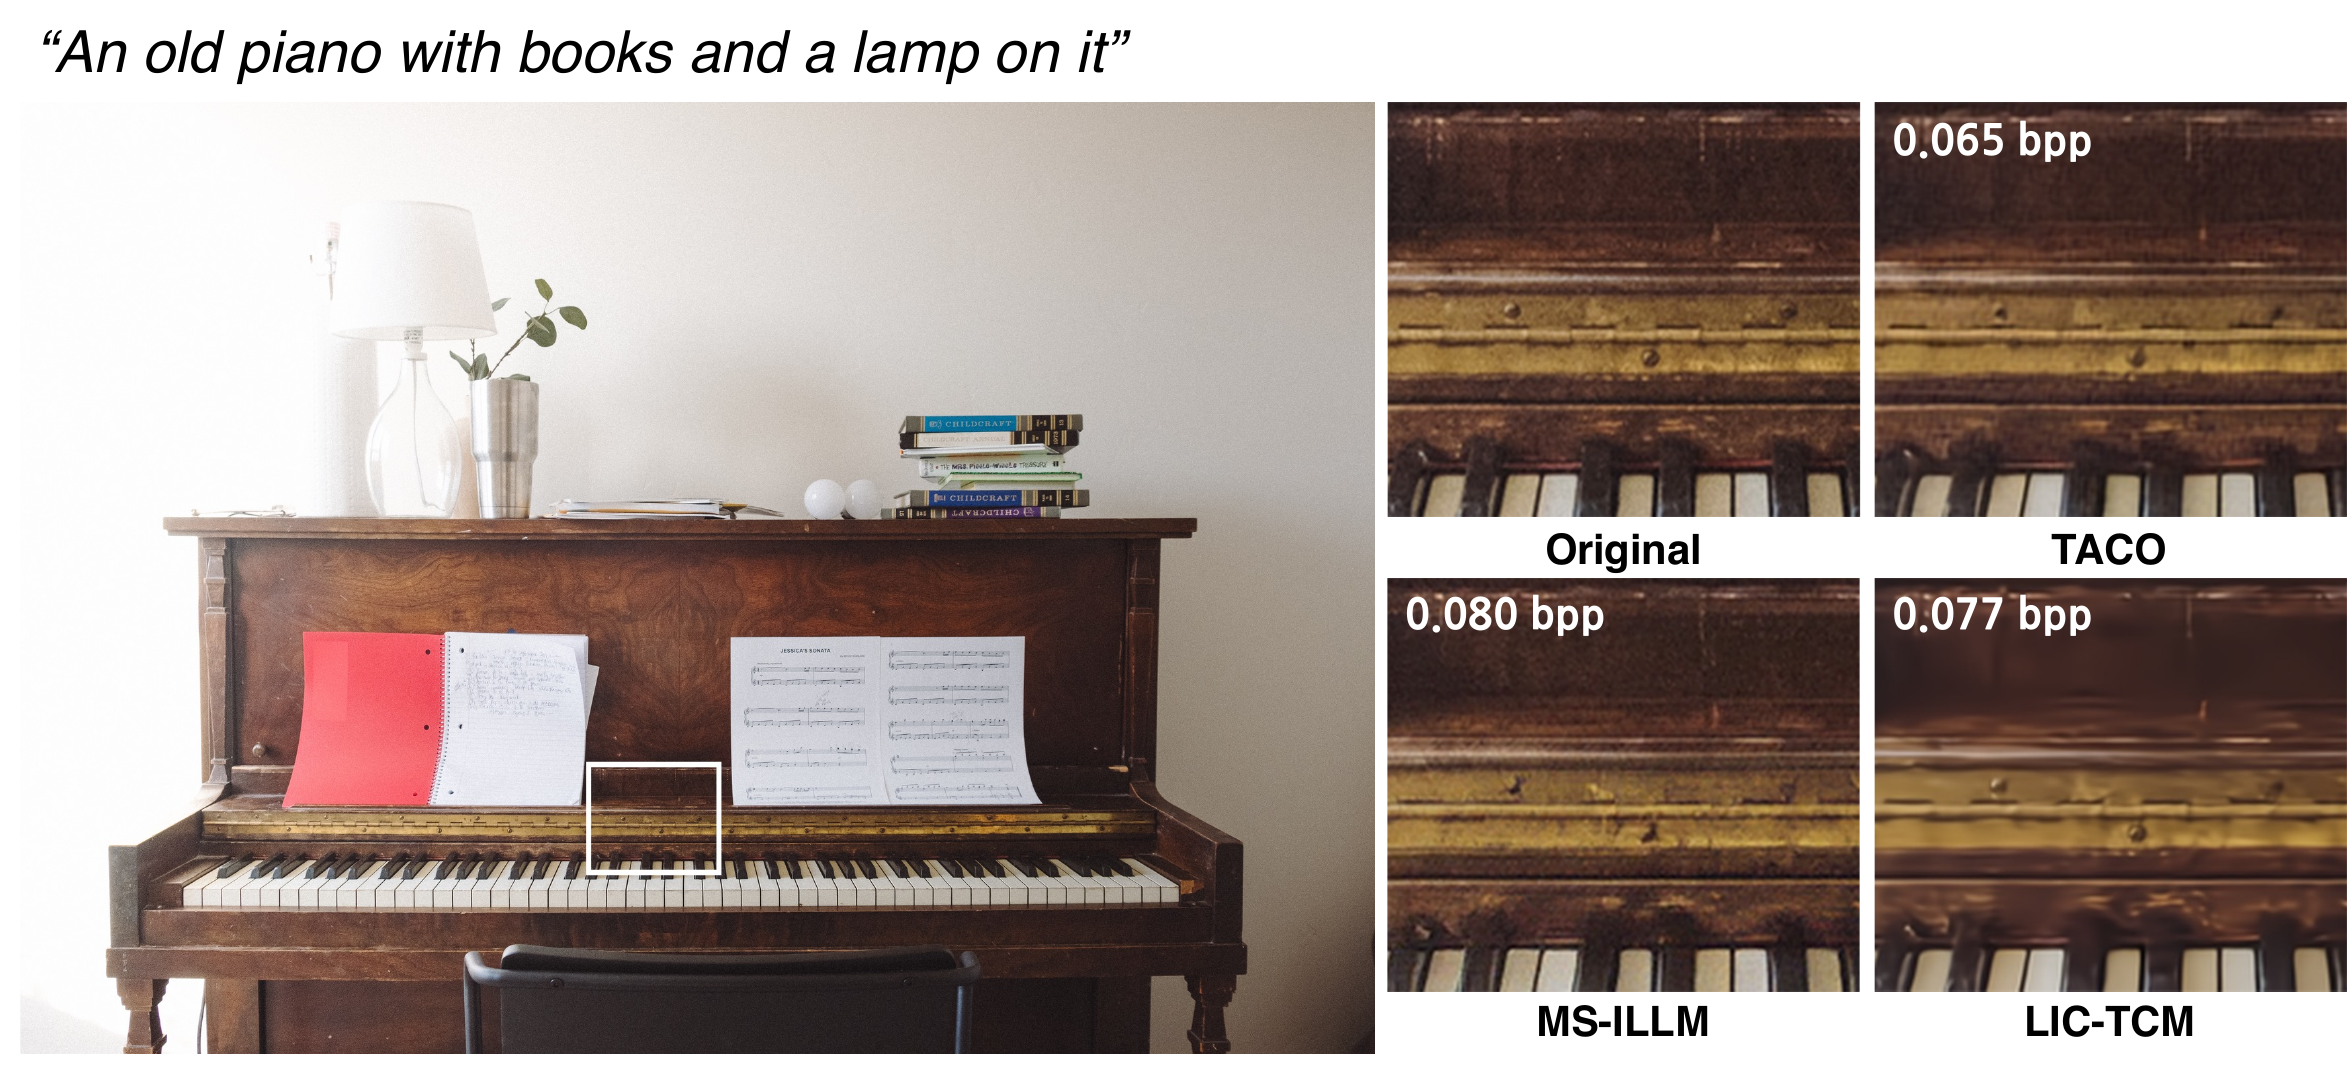}}
    \caption{ \textbf{Qualitative results.} TACO reconstructs the fine details of original image; see the {\color{red} gold hinge part}  }
    \label{fig:appendix_qualitative_piano} 
\end{figure*}
